# Supplementary material for: Polaronic high-temperature superconductivity in optimally doped bismuthate Ba0:63K0:37BiO3
Source: arXiv:1410.4100 source file (2014-10-14)
Supplement: Supplementary file 1 [file PRL-BKBO-SM-R1.pdf]

# Supplemental Material: Polaronic high-temperature superconductivity in optimally doped bismuthate $Ba_{0.63}K_{0.37}BiO_3$

N. Derimow[1], J. Labry[1], A. Khodagulyan[1], J. Wang[2], and Guo-meng Zhao[1,*]

[1]*Department of Physics and Astronomy, California State University, Los Angeles, CA 90032, USA*

[2] *Department of Physics, Faculty of Science, Ningbo University, Ningbo, P. R. China*

## I. Procedure for preparing optimally doped bismuthate superconductor $Ba_{0.63}K_{0.37}BiO_3$

Well-ground powder mixture of $K_2CO_3$ (99.995%), $BaCO_3$ (99.999%), and $Bi_2O_3$ (99.999%) were placed in a covered ceramic crucible and heated to 720°C in vacuum within 40 minutes. After reacting at 720 °C in vacuum for 2 hours (the system was continuously pumped by a mechanical pump to keep a high vacuum), the sample was cooled rapidly to 100 °C for about 5 minutes. After cooling the system to room temperature, pure oxygen gas was filled into the system and the sample was annealed in 1 bar oxygen gas at 450 °C for 30 minutes and cooled down to room temperature within 40 minutes.

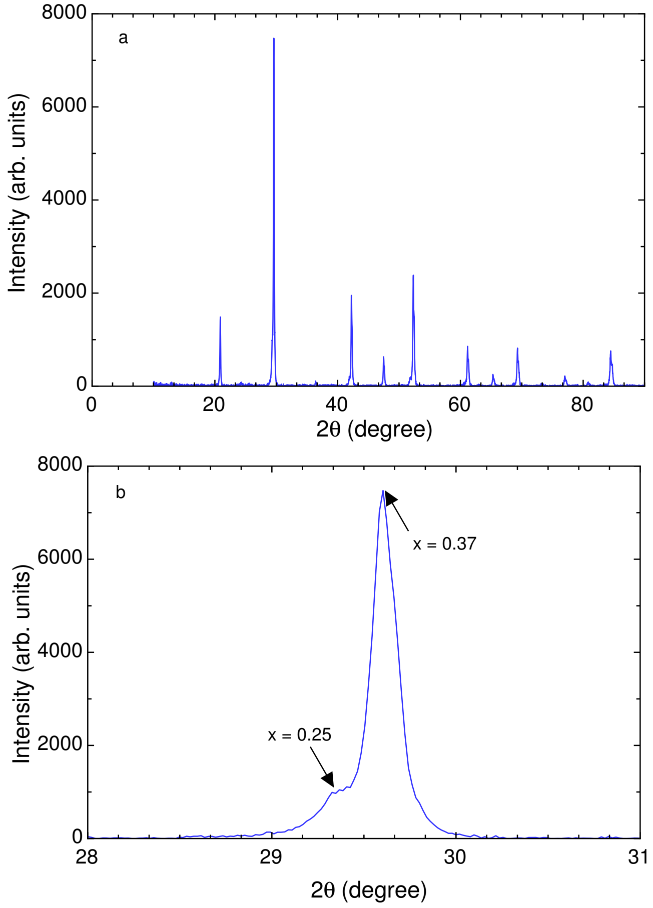


FIG. 1: a) X-ray diffraction spectrum of $Ba_{1-x}K_xBiO_3$. b) Zoomed view of the (110) peak of the cubic phase. The arrows mark the positions expected for the compositions.

X-ray diffraction spectrum (Fig. 1) indicates that the sample contains a majority superconducting phase of $Ba_{0.63}K_{0.37}BiO_3$ and a minority nonsuperconducting phase of $Ba_{0.75}K_{0.25}BiO_3$. No other impurity phase is visible in the X-ray diffraction spectrum.

## II. Determination of the electronic Sommerfeld coefficient $\gamma$ for the bismuthate superconductor $\mathbf{Ba_{0.63}K_{0.37}BiO_3}$

From the unbiased parameters: $\lambda(0) = 198.5$ nm, $H_{c2}(0) = 330.5$ kOe, and $k_B T_c/\hbar\omega_{\rm ln} = 0.107$, we can determine the electronic Sommerfeld coefficient $\gamma$, Ginzburg-Landau parameter $\kappa$, and the specific-heat jump $\Delta C$ at $T_c$ using the standard expressions for the conventional strong-coupling superconductors. Assuming that $Ba_{0.63}K_{0.37}BiO_3$ is a clean superconductor, as justified below, and using $k_B T_c/\hbar\omega_{\rm ln} = 0.107$ and empirical formulas for conventional superconductors [1], we determine the slope $dH_{c2}/dT$ and $d(\Phi_0/\lambda^2)/dT$ near $T_c$ to be $1.344 H_{c2}(0)/T_c$ and $2.882\Phi_0/[\lambda^2(0)T_c]$, respectively. The specific heat hump $\Delta C/\gamma T_c$ is calculated to be 2.416 with $k_B T_c/\hbar\omega_{\rm ln} = 0.107$. Using $\lambda(0) = 198.5$ nm and $H_{c2}(0) = 330.5$ kOe and the above relations, we obtain $d(\Phi_0/\lambda^2)/dT = -47.3$ Oe/K and $dH_{c2}/dT = -13880$ Oe/K. We then determine $\kappa = 42.92$ using the standard expressions [2]: $2\kappa^2/\ln\kappa = (dH_{c2}/dT)/(dH_{c1}/dT)$ and $dH_{c1}/dT = (\ln\kappa/4\pi)[d(\Phi_0/\lambda^2)/dT]$. Finally from $\Delta C/T_c = (1/8\pi\kappa^2)(dH_{c2}/dT)^2$ (Ref. [3]) and $\Delta C/\gamma T_c = 2.416$, we find $\Delta C/T_c = 19.77$ mJ/moleK$^2$ and $\gamma = 8.18$ mJ/moleK$^2$.

## III. The total zero-temperature mass enhancement factor $f_t$ in $\mathbf{Ba_{1-x}K_xBiO_3}$

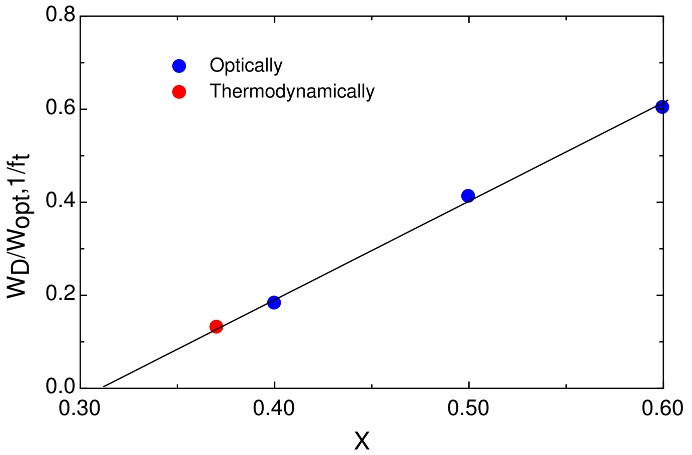


FIG. 2: Theoretically calculated [5] Drude weight, $W_D$, normalized by total optical weight $W_{opt}$, as a function of the doping level $x$ together with $1/f_t$ for $x = 0.37$, which is inferred from the thermodynamical quantities.

From the inferred $\gamma = 8.18$ mJ/moleK$^2$ and the bare Sommerfeld coefficient $\gamma_b = 1.08$ mJ/molK$^2$ [4], we calculate the total zero-temperature mass enhancement factor $f_t = \gamma/\gamma_b$

= 7.54. The total mass enhancement factor can be also deduced from optical conductivity [5], that is, $f_t = W_{opt}(g=0)/W_D(g)$, where $W_{opt}(g=0)$ is the total optical weight without electron-phonon coupling and $W_D(g)$ is the Drude weight in the presence of electron-phonon coupling. In Fig. 2, we plot the theoretically calculated [5] Drude weight, $W_D$, normalized by total optical weight $W_{opt}$, as a function of the doping level $x$ together with $1/f_t$ for $x = 0.37$, which is inferred from the thermodynamical quantities. From the figure, it is apparent that our inferred mass enhancement factor $f_t$ is in quantitative agreement with the theoretical prediction [5].

## IV. Superconducting fluctuation in $Ba_{1-x}K_xBiO_3$

The inferred $\Delta C/T_c = 19.77$ mJ/moleK$^2$ is over one order of magnitude larger than the specific-heat anomaly observed earlier [6, 7]. This inconsistency can be explained in terms of a higher-order superconducting phase transition [8, 9]. Considering a weak superconducting fluctuation for a second-order phase transition, the free energy can be written as $F(T) = -f_0(1 - T/T_c)^{2-\alpha}$, where $\alpha$ is a small number which can be calculated by pseudo-perturbative schemes (such as Gaussian approximation) [8]. However, when the superconducting fluctuation is large, the magnitude of $\alpha$ should be large and beyond the realm of a perturbative approach. Then the unperturbed ground state could be a transition of order corresponding to the nearest integer, that is, a third order or even a fourth order depending on how large is the superconducting fluctuation. A very small $\Delta C/T_c$ value observed earlier [6, 7] is consistent with a fourth order phase transition, as clearly demonstrated by experiments [8, 9].

On the other hand, the specific-heat measurement on a high-quality single-crystalline sample [10] showed a much larger specific-heat anomaly, that is, $\Delta C/T_c \simeq 6$ mJ/moleK$^2$, which is about 30% of the above inferred value. This implies that the superconducting fluctuation in this crystal should be much smaller than in the other samples, but still substantial. We can check the critical behaviors to see how large is the superconducting fluctuation in this crystal. In Fig. 3a, we display the upper critical fields near $T_c$, which were determined by specific heat measurements [10]. It is apparent that $H_{c2} \propto (1 - T/T_c)^p$ with $p = 1.33\pm0.04$. In Fig. 3b, we plot $dM_{rev}/d\ln H$ ($\propto H_{c1}$) as a function of $(1 - T/T_c)$ near $T_c$. The solid line is the curve proportional to $(1 - T/T_c)^q$ with $q = 1.59\pm0.03$. The values of the $p$ and $q$ imply that $F(T) \propto (1 - T/T_c)^{2-\alpha}$ with $\alpha = -0.92\pm0.07$. The value of $\alpha \simeq -1.0$ suggests a large superconducting fluctuation, which would lead to a third-order phase transition. The

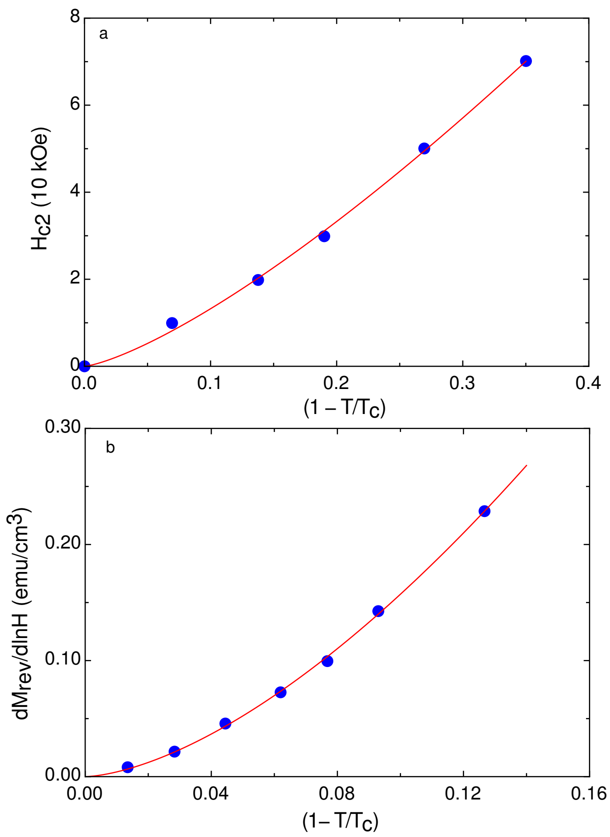


FIG. 3: a) Upper critical field as a function of $(1 - T/T_c)$ for the crystal. The data were taken from Ref. [10]. The solid line is the curve proportional to $(1 - T/T_c)^p$ with $p$ = 1.33±0.04. b) $dM_{rev}/d\ln H$ versus $(1 - T/T_c)$ for the crystal (where $M_{rev}$ is the reversible magnetization). The data were taken from Ref. [10]. The solid line is the curve proportional to $(1 - T/T_c)^q$ with $q$ = 1.59±0.03.

fourth order superconducting transition found in other crystals [8, 9] may be due to the fact that those crystals have more disorders, leading to a larger superconducting fluctuation.

We can also check the superconducting fraction of this crystal from the measured $dM_{rev}/d\ln H$ down to $0.55T_c$ (Ref. [10]), as shown in Fig. 4. The solid line is the theoretical curve calculated for a clean superconductor with $k_BT_c/\hbar\omega_{\ln} = 0.115$ (Ref. [1]). The extrapolated zero-temperature value of $dM_{rev}/d\ln H$ is 0.87 emu/cm$^3$, which leads to $f_{sc}$ = 67.9% when $\lambda(0)$ = 198.5 nm and Eq. 2 of the main text is used. The superconducting fraction in this high-quality crystal is very close to that (69.4%) in our polycrystalline sample. With the correction of the superconducting fraction, the measured $\Delta C/T_c$ for the superconducting phase is about 8.8 mJ/moleK$^2$, which is about 45% of the above inferred value of 19.77 mJ/moleK$^2$. The 55% suppression of $\Delta C/T_c$ should arise from the large

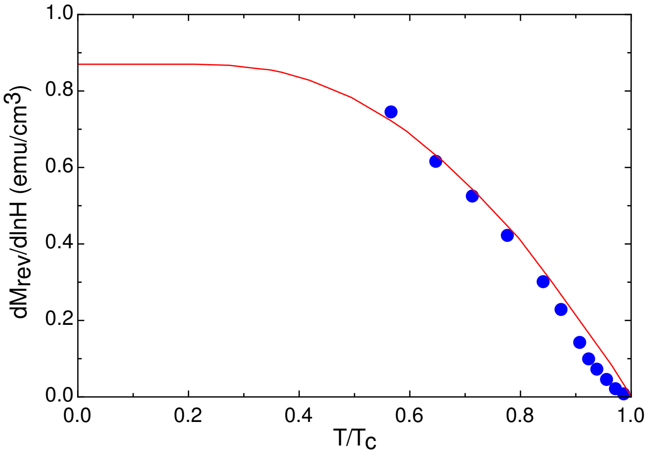


FIG. 4: $dM_{rev}/d\ln H$ as a function of $T/T_c$ for the crystal [10]. The solid line is the theoretical curve calculated for a clean superconductor with $k_BT_c/\hbar\omega_{\ln} = 0.115$ (Ref. [1]). The extrapolated zero-temperature value of $dM_{rev}/d\ln H$ is 0.87 emu/cm$^3$.

superconducting fluctuation, as evidenced from the large $\alpha$ value.

### V. Bare plasma energy in $Ba_{0.6}K_{0.4}BiO_3$

The coherence length near $T_c$ within the BCS model is given by [11] $\xi(T) = 0.74\xi_{BCS}\sqrt{G(0.882\xi_{BCS}/l)}/\sqrt{1-T/T_c}$, where $G(x)$ is the Gor'kov function defined by $G(x) = \sum_{n=0}^{\infty}\frac{0.95}{(1+2n)^2(1+2n+x)}$, $\xi_{BCS} = \frac{\hbar v_F^{**}}{\pi\Delta(0)}$, and the effective Fermi velocity $v_F^{**}$ is simply equal to the bare Fermi velocity $v_F$. Due to strong electron-boson coupling, $v_F^{**}$ is reduced by a factor of $f_t$ compared with $v_F$, which is calculated to be $1.08\times10^6$ m/s for $Ba_{0.6}K_{0.4}BiO_3$ (Ref. [12]). Because of strong electron-boson coupling, the slope of the upper critical field near $T_c$ is modified as [13]

$$\frac{dH_{c2}}{dT} = -\frac{\phi_0}{2\pi T_c}\frac{\eta_{H_{c2}}(T_c)}{0.74^2\xi_{BCS}^2G(0.882\xi_{BCS}/l)}, \tag{1}$$

where $\eta_{H_{c2}}(T_c) = 1.18$ for a clean superconductor with $k_BT_c/\hbar\omega_{\ln} = 0.107$ (Ref. [1]). Substituting $\Delta(0) = 5.95$ meV, $v_F = 1.08\times10^6$ m/s, and $f_t = 7.54$ into $\xi_{BCS} = \frac{\hbar v_F}{f_t\pi\Delta(0)}$ yields $\xi_{BCS} = 50.6$ Å. Substituting $\xi_{BCS} = 50.6$ Å, $dH_{c2}/dT =$ -13880 Oe/K, and $\eta_{H_{c2}}(T_c) = 1.18$ into Eq. 1, we get $l = 70.77$ Å. The fact that $l > \xi_{BCS}$ implies that the $Ba_{0.6}K_{0.4}BiO_3$ is a rather clean superconductor. Finally the bare plasma energy $\hbar\Omega_p$ is calculated to be 3.75 eV from the relation: $\hbar\Omega_p = [\hbar c/\lambda(0)]\sqrt{f_t(1+(\pi^2/8)\xi_{BCS}/l)}$ (see Eq. 145 of Ref. [14]) and $\lambda(0) = 198.5$ nm. The inferred bare plasma energy of 3.75 eV is slightly smaller than the value (4.03 eV) predicted from the first-principle calculation [12]. Since charge carriers in

the band edge can be localized by random potential arising from dopants and/or defects, the free carrier density should be lower than the total carrier density.

* gzhao2@calstatela.edu

---

[1] J. P. Carbotte, Rev. Mod. Phys. **62**, 1027 (1990).

[2] M. Tinkham, *Introduction to Superconductivity*, (McGraw-Hill, New York, 1996).

[3] W. K. Kwok *et al.*, Phys. Rev. B **40**, 9400 (1989).

[4] L. F. Mattheiss and D. R. Hamann, Phys. Rev. Lett. **60**, 2681 (1988).

[5] R. Nourafkan, F. Marsiglio, and G. Kotliar, Phys. Rev. Lett. **109** , 017001 (2012).

[6] J. E. Graebner, L. F. Schneemeyer, and J. K. Thomas, Phys. Rev. B **39**, 9682 (1989).

[7] B. F. Woodfield, D. A. Wright, R. A. Fisher, N. E. Philips, and H.Y. Tang, Phys. Rev. Lett. **83**, 4622 (1999).

[8] P. Kumar, D. Hall, and R. G. Goodrich, Phys. Rev. Lett., **82**, 4532 (1999).

[9] D. Hall, R. G. Goodrich, C. G. Grenier, P. Kumar, M. Chaparala, and M. L. Norton, arXiv: cond-mat/9912160.

[10] S. Blanchard, T. Klein, J. Marcus, I. Joumard, A. Sulpice, P. Szabo, P. Samuely, A. G. M. Jansen, and C. Marcenat, Phys. Rev. Lett. **88**, 177201 (2002).

[11] J. R. Tucker and B. I. Halperin, Phys. Rev. B **3**, 3768 (1971).

[12] L. F. Mattheiss, Phys. Rev. B **28**, 6629 (1983).

[13] T. P. Orlando, E. J. McNiff, Jr., S. Foner, and M. R. Beasley, Phys. Rev. B **19**, 4545 (1979).

[14] F. Marsiglio and J.P. Carbotte, arXiv:cond-mat/0106143v1.
